# Supplementary material for: Extract and Characterize Hairpin Vortices in Turbulent Flows
Source: arXiv:2308.06283 source file (2023-11-08)
Supplement: Supplementary file 1 [file supplemental.tex]

\setcounter{section}{0}
\setcounter{figure}{0}
\setcounter{table}{0}
\setcounter{equation}{0}
\section{Description of the Flow Datasets}
A brief description of the flow datasets used in our experiments reported in Table 2 (of the paper) is given below. 
\subsection{B\'enard Flow}
The B\'enard flow dataset simulates Rayleigh-B\'enard convection between two parallel horizontal planes. It represents the phenomenon where a fluid heated from below in a gravitational field displays upward and downward flow currents, forming the characteristic circulation pattern known as B\'enard convection or cells. Overview of the B\'enard flow is shown in \cref{fig:benard.supp}.

\begin{figure}[h]
 \centering % avoid the use of \begin{center}...\end{center} and use \centering instead (more compact)
 \includegraphics[width=0.95\linewidth]{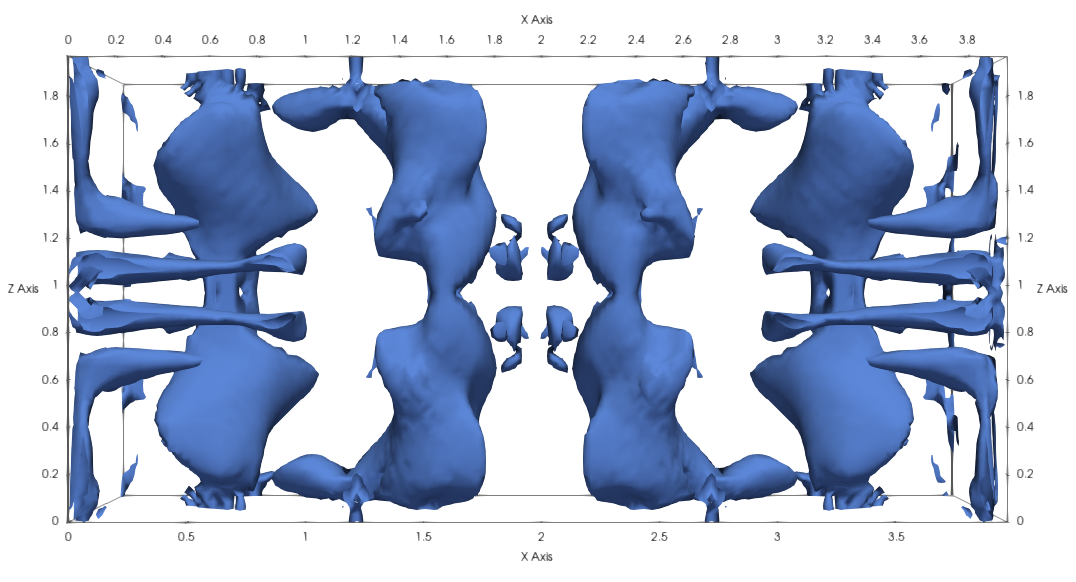}
 %\vskip -2pt
 \caption{This figure shows the visualization of B\'enard flow dataset using the vortex extraction method. Vortices are extracted using $\lambda_2$ method with the threshold value of $-4.0$.}
 \label{fig:benard.supp}
\end{figure}

\subsection{Cylinder Flow}
Cylinder flow is the simulation of flow behind a cylinder. It refers to the fluid dynamics phenomenon that occurs when a fluid flows past a solid cylinder, resulting in the formation of vortices. These vortices include a distinct pattern of primary vortex shedding in the wake of the cylinder. Overview of the cylinder flow dataset is shown in \cref{fig:cylinder.supp}.

\begin{figure}[h]
 \centering % avoid the use of \begin{center}...\end{center} and use \centering instead (more compact)
 \includegraphics[width=0.95\linewidth]{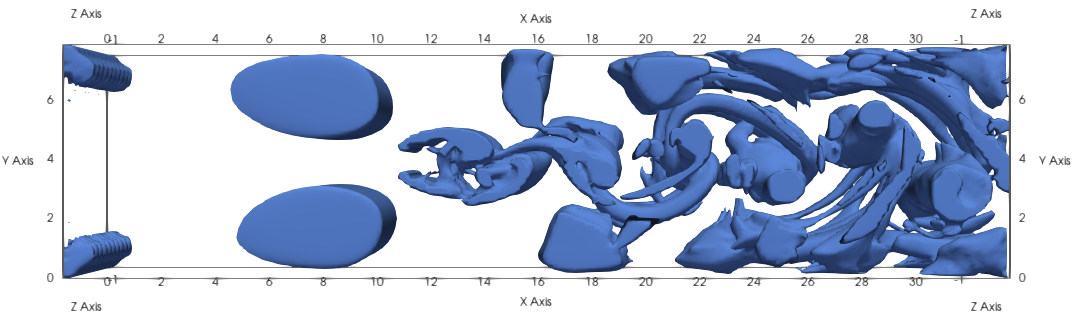}
 %\vskip -2pt
 \caption{This figure shows the visualization of cylinder flow dataset using the vortex extraction method. Vortices are extracted using $\lambda_2$ method with the threshold value of $-0.002$.}
 \label{fig:cylinder.supp}
\end{figure}

\subsection{Crayfish Flow}
This dataset represents the simulation of heat flow around a cooking crayfish which focuses on analyzing heat behavior and distribution during the cooking process. Various vortices form near the crayfish surface, in its wake, and due to heating-induced convection currents. These vortices play a crucial role in heat distribution and flow patterns during crayfish cooking. Overview of the crayfish flow dataset is shown in \cref{fig:crayfish.supp}.

\begin{figure}[h]
 \centering % avoid the use of \begin{center}...\end{center} and use \centering instead (more compact)
 \includegraphics[width=0.95\linewidth]{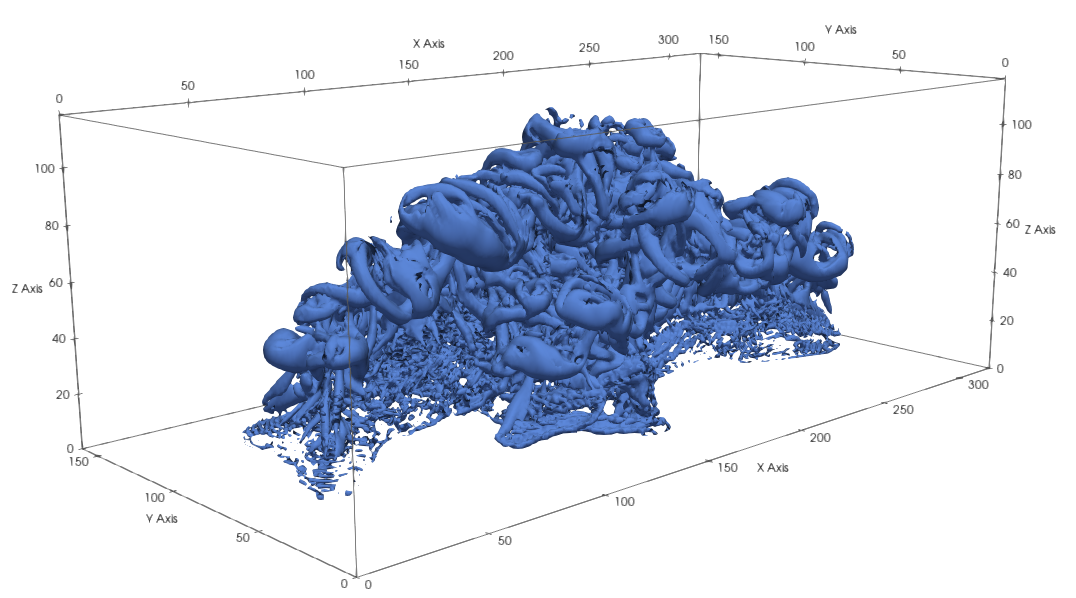}
 %\vskip -2pt
 \caption{This figure shows the visualization of crayfish flow dataset using the vortex extraction method. Vortices are extracted using $\lambda_2$ method with the threshold value of $-5e^{-4}$.}
 \label{fig:crayfish.supp}
\end{figure}

\subsection{Plume Flow}
This dataset refers to the simulation of a compressible downflow solar plume. The compressible downflow solar plume is a column of hot, compressed gas that descends from a high-temperature region in the solar atmosphere, resulting from convective motion and heating of solar material. It has a substantial impact on energy transport and dynamics in the Sun's outer layers. Overview of the plume flow dataset is shown in \cref{fig:plume.supp}.

\begin{figure}[h]
 \centering % avoid the use of \begin{center}...\end{center} and use \centering instead (more compact)
 \includegraphics[width=0.95\linewidth]{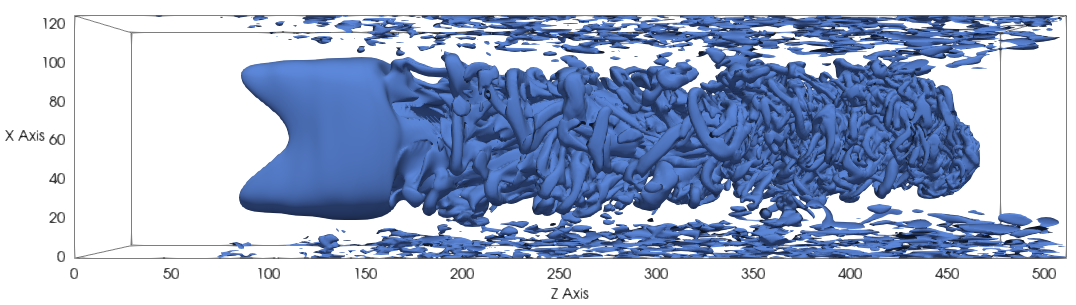}
 %\vskip -2pt
 \caption{This figure shows the visualization of plume flow dataset using the vortex extraction method. Vortices are extracted using $\lambda_2$ method with the threshold value of $-5e^{-7}$.}
 \label{fig:plume.supp}
\end{figure}

\subsection{Couette Flow}
A couette flow is the flow of a viscous fluid between two parallel plates, with one plate moving relative to the other. No-slip boundary condition assumes zero velocity at the solid surface, while the free-slip boundary condition assumes no shear stress or tangential velocity at the surface. The dataset is the simulation of a couette flow at a relatively high Reynolds number of 180 to study the effect of turbulence at no-slip (\emph{bottom}) and free-slip (\emph{top}) boundaries. Overview of the couette  flow dataset is shown in Figure 1 of the main paper.

\section{Description of the Variables in Table 1}
Given $\vec{v}$, the fluid \textbf{Velocity} at each point in the dataset, the \textbf{Jacobian} $\mathbf{J}$ is the spatial derivatives of the velocity, and \textbf{acceleration} $\vec{a}$ is defined as $\vec{a}=\textbf{J}\vec{v}$.

\noindent \textbf{Vorticity} is the curl of velocity, defined as $\vec{\omega} = \nabla \times \vec{v}$ where $\nabla$ is nabla or del operator. 

\noindent \textbf{Enstrophy} $\xi$ is a scalar to quantify the vortex strength and is calculated as $\xi = \frac{\vec{\omega}.\vec{\omega}}{2}$. 

\noindent \textbf{Spanwise Vorticity Fluctuations} $\omega_{y}'$ is the turbulent fluctuation of the instantaneous vorticity $\omega_{y}$, where $\omega_{y}$ is the component of the vorticity $\vec{\omega}$ in y-direction, assuming 'y' is the spanwise direction of the flow. $\omega_{y}'$ is calculated as $\omega_{y}' = \omega_{y} - \left<\omega_{y}\right>$, where $\left<\omega_{y}\right>$ is the time and horizontal average of $\omega_{y}$. 

\noindent \textbf{Divergence} "$Div$" refers to a scalar quantity that represents the expansion or contraction of fluid flow at a given point. It is calculated as $Div(\vec{v}) = \nabla.\vec{v}$. 

\noindent By decomposing Jacobian $\textbf{J}$ into the strain rate tensor $S$ and the vorticity tensor $\Omega$, the $\textbf{Q}$-criterion is calculated as follows \cref{eq_supp.1}.
    \begin{equation}
    \label{eq_supp.1}
        S = \frac{\textbf{J} + \textbf{J}^T}{2} \qquad \Omega = \frac{\textbf{J} - \textbf{J}^T}{2}, \qquad Q = \frac{1}{2}\left(\left|\Omega\right|^2 - \left|S\right|^2 \right)
    \end{equation}
For vortical regions $Q>0$.

\noindent ${\Delta}$-criterion is derived from $Q$-criterion and the determinant of Jacobian $\mathbf{J}$ as shown in \cref{eq_supp.2}.
    \begin{equation}
    \label{eq_supp.2}
        \Delta = \left(\frac{Q}{3}\right)^3 + \left(\frac{det(\textbf{J})}{2}\right)^2
    \end{equation}
For vortical regions, $\Delta>0$.

\noindent Denote by $\lambda_1 \geq \lambda_2 \geq \lambda_3$, the real eigenvalues of the symmetric tensor $S^2$+$\Omega^2$ sorted in the descending order. Then $\mathbf{\lambda_2}$-criterion refers to the second largest eigenvalue in the order satisfying
    \begin{equation}
    \label{eq_supp.3}
        \lambda_2 (S^2+\Omega^2) < 0
    \end{equation}
For vortical regions, $\lambda_2<0$.

\noindent $\mathbf{\lambda_{ci}}$-criterion refers to the imaginary parts of the complex conjugate-eigenvalues $\lambda_{cr} \pm \iota \lambda_{ci}$ of the Jacobian $\textbf{J}$. For vortical regions, $\lambda_{ci}$ exhibits a large value. Additional details on the computation of the above attributes are provided in~\cite{gunther2018state}.

\section{Stages of the Hairpin Vortex}

\begin{figure}[t]
 \centering % avoid the use of \begin{center}...\end{center} and use \centering instead (more compact)
 \includegraphics[width=0.95\linewidth]{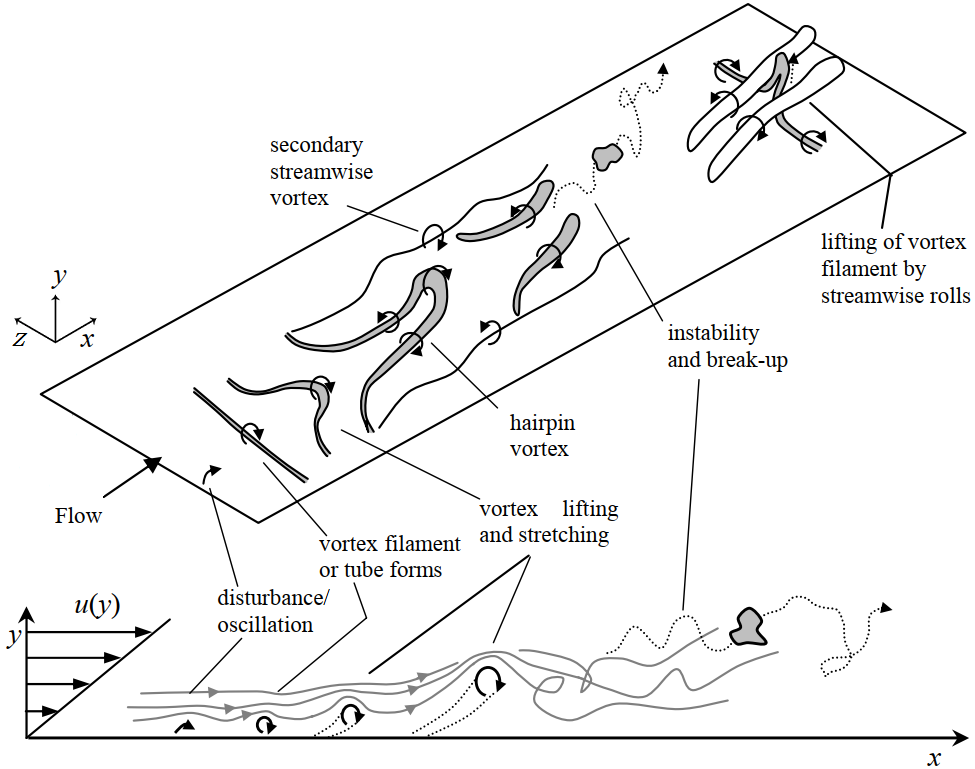}
 %\vskip -2pt
 \caption{This figure shows three stages in the lifespan of a hairpin vortex. The x-axis represent the flow/streamwise direction, the z-axis represent the spanwise direction and the y-axis represents the height or the perpendicular direction.}
 \label{fig:hairpin_stages}
\end{figure}

Different stages of the life span of a hairpin are illustrated in \cref{fig:hairpin_stages}. A spanwise vortex tube forms the $\Omega$ shape vortex because of the vortex lifting and stretching, which we refer to as stage (a) in section 6 of the main paper. The stage (b) is referred to the fully developed hairpin vortex and stage (c) is referred to the instability and break-up of the hairpin vortex, respectively.
