# Supplementary material for: Extract and Characterize Hairpin Vortices in Turbulent Flows
Source: arXiv:2308.06283 ancillary file (2023-11-08)
Supplement: Supplementary file 2 [file Supplemental_doc.pdf]

# Extract and Characterize Hairpin Vortices in Turbulent Flows - Supplemental Document

Adeel Zafar 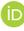, Di Yang 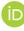, Guoning Chen 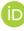

**Abstract**—This supplemental document describes the individual flow datasets used in this work. It also describes how the individual attributes included in the profile of a vortex are calculated. In addition, it illustrates the different stages of a hairpin vortex in its life span.

**Index Terms**—Turbulent flow, vortices, hairpin vortex extraction

## 1 DESCRIPTION OF THE FLOW DATASETS

A brief description of the flow datasets used in our experiments reported in Table 2 (of the paper) is given below.

### 1.1 Bénard Flow

The Bénard flow dataset simulates Rayleigh-Bénard convection between two parallel horizontal planes. It represents the phenomenon where a fluid heated from below in a gravitational field displays upward and downward flow currents, forming the characteristic circulation pattern known as Bénard convection or cells. Overview of the Bénard flow is shown in Fig. 1.

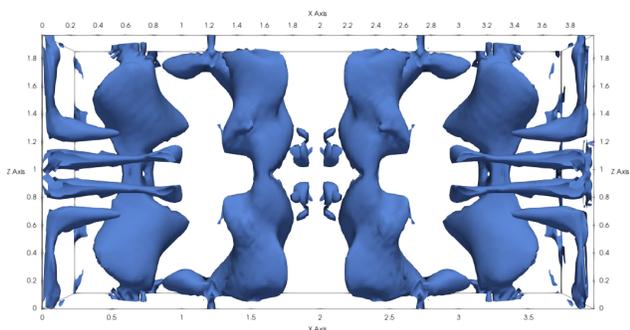

Fig. 1: This figure shows the visualization of Bénard flow dataset using the vortex extraction method. Vortices are extracted using  $\lambda_2$  method with the threshold value of  $-4.0$ .

### 1.2 Cylinder Flow

Cylinder flow is the simulation of flow behind a cylinder. It refers to the fluid dynamics phenomenon that occurs when a fluid flows past a solid cylinder, resulting in the formation of vortices. These vortices include a distinct pattern of primary vortex shedding in the wake of the cylinder. Overview of the cylinder flow dataset is shown in Fig. 2.

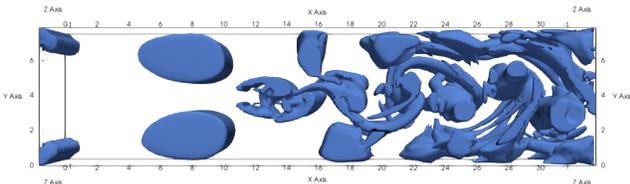

Fig. 2: This figure shows the visualization of cylinder flow dataset using the vortex extraction method. Vortices are extracted using  $\lambda_2$  method with the threshold value of  $-0.002$ .

### 1.3 Crayfish Flow

This dataset represents the simulation of heat flow around a cooking crayfish which focuses on analyzing heat behavior and distribution during the cooking process. Various vortices form near the crayfish surface, in its wake, and due to heating-induced convection currents. These vortices play a crucial role in heat distribution and flow patterns during crayfish cooking. Overview of the crayfish flow dataset is shown in Fig. 3.

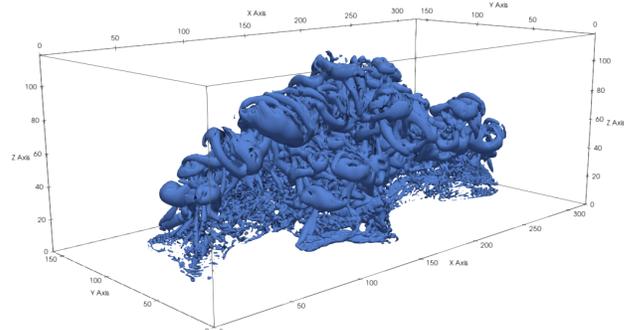

Fig. 3: This figure shows the visualization of crayfish flow dataset using the vortex extraction method. Vortices are extracted using  $\lambda_2$  method with the threshold value of  $-5e^{-4}$ .

### 1.4 Plume Flow

This dataset refers to the simulation of a compressible downflow solar plume. The compressible downflow solar plume is a column of hot, compressed gas that descends from a high-temperature region in the solar atmosphere, resulting from convective motion and heating of solar material. It has a substantial impact on energy transport and dynamics in the Sun's outer layers. Overview of the plume flow dataset is shown in Fig. 4.

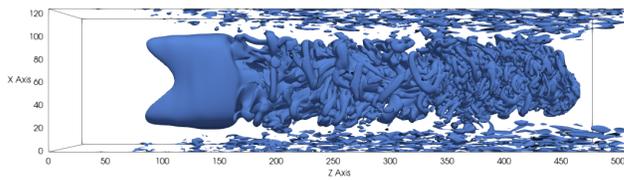

Fig. 4: This figure shows the visualization of plume flow dataset using the vortex extraction method. Vortices are extracted using  $\lambda_2$  method with the threshold value of  $-5e^{-7}$ .

### 1.5 Couette Flow

A couette flow is the flow of a viscous fluid between two parallel plates, with one plate moving relative to the other. No-slip boundary condition assumes zero velocity at the solid surface, while the free-slip boundary condition assumes no shear stress or tangential velocity at the surface. The dataset is the simulation of a couette flow at a relatively high Reynolds number of 180 to study the effect of turbulence at no-slip

• Adeel Zafar, Di Yang, and Guoning Chen are with the University of Houston. E-mail: azafar3@uh.edu, diyang@uh.edu, gchen16@uh.edu

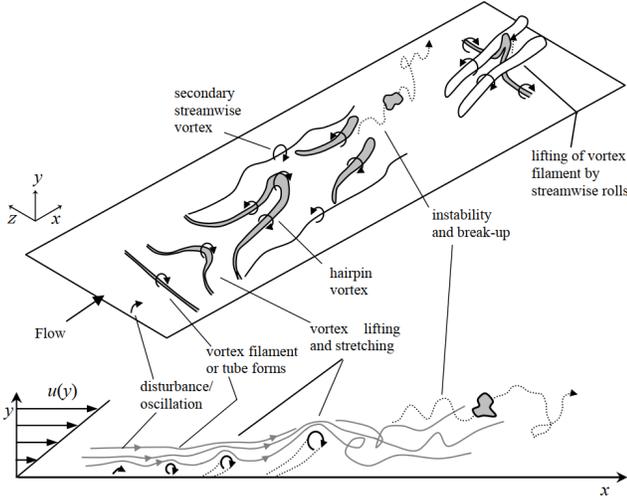

Fig. 5: This figure shows three stages in the lifespan of a hairpin vortex. The x-axis represent the flow/streamwise direction, the z-axis represent the spanwise direction and the y-axis represents the height or the perpendicular direction.

(bottom) and free-slip (top) boundaries. Overview of the couette flow dataset is shown in Figure 1 of the main paper.

## 2 DESCRIPTION OF THE VARIABLES IN TABLE 1

Given  $\vec{v}$ , the fluid **Velocity** at each point in the dataset, the **Jacobian J** is the spatial derivatives of the velocity, and **acceleration**  $\vec{a}$  is defined as  $\vec{a} = \mathbf{J}\vec{v}$ .

**Vorticity** is the curl of velocity, defined as  $\vec{\omega} = \nabla \times \vec{v}$  where  $\nabla$  is nabla or del operator.

**Enstrophy**  $\xi$  is a scalar to quantify the vortex strength and is calculated as  $\xi = \frac{\vec{\omega} \cdot \vec{\omega}}{2}$ .

**Spanwise Vorticity Fluctuations**  $\omega'_y$  is the turbulent fluctuation of the instantaneous vorticity  $\omega_y$ , where  $\omega_y$  is the component of the vorticity  $\vec{\omega}$  in y-direction, assuming 'y' is the spanwise direction of the flow.  $\omega'_y$  is calculated as  $\omega'_y = \omega_y - \langle \omega_y \rangle$ , where  $\langle \omega_y \rangle$  is the time and horizontal average of  $\omega_y$ .

**Divergence** "Div" refers to a scalar quantity that represents the expansion or contraction of fluid flow at a given point. It is calculated as  $Div(\vec{v}) = \nabla \cdot \vec{v}$ .

By decomposing Jacobian **J** into the strain rate tensor **S** and the vorticity tensor **Ω**, the **Q-criterion** is calculated as follows Eq. (1).

$$S = \frac{\mathbf{J} + \mathbf{J}^T}{2}, \quad \Omega = \frac{\mathbf{J} - \mathbf{J}^T}{2}, \quad Q = \frac{1}{2} (|\Omega|^2 - |S|^2) \quad (1)$$

For vortical regions  $Q > 0$ .

$\Delta$ -criterion is derived from **Q-criterion** and the determinant of Jacobian **J** as shown in Eq. (2).

$$\Delta = \left(\frac{Q}{3}\right)^3 + \left(\frac{\det(\mathbf{J})}{2}\right)^2 \quad (2)$$

For vortical regions,  $\Delta > 0$ .

Denote by  $\lambda_1 \geq \lambda_2 \geq \lambda_3$ , the real eigenvalues of the symmetric tensor  $S^2 + \Omega^2$  sorted in the descending order. Then  $\lambda_2$ -criterion refers to the second largest eigenvalue in the order satisfying

$$\lambda_2(S^2 + \Omega^2) < 0 \quad (3)$$

For vortical regions,  $\lambda_2 < 0$ .

$\lambda_{ci}$ -criterion refers to the imaginary parts of the complex conjugate-eigenvalues  $\lambda_{cr} \pm i\lambda_{ci}$  of the Jacobian **J**. For vortical regions,  $\lambda_{ci}$  exhibits a large value. Additional details on the computation of the above attributes are provided in [1].

## 3 STAGES OF THE HAIRPIN VORTEX

Different stages of the life span of a hairpin are illustrated in Fig. 5. A spanwise vortex tube forms the  $\Omega$  shape vortex because of the vortex lifting and stretching, which we refer to as stage (a) in section 6 of the main paper. The stage (b) is referred to the fully developed hairpin

vortex and stage (c) is referred to the instability and break-up of the hairpin vortex, respectively.

## FIGURE CREDITS

Figure 5 is taken from [2].

## ACKNOWLEDGMENTS

We thank the anonymous reviewers for their valuable feedback. This research was supported by NSF OAC 2102761.

## REFERENCES

- [1] T. Günther and H. Theisel. The state of the art in vortex extraction. *Computer Graphics Forum*, 37(6):149–173, 2018. doi: 10.1111/cgf.13319 2
- [2] L. M. Jiji. Convection in external turbulent flow. In *Heat Convection: Second Edition*, pp. 293–360. Springer Berlin Heidelberg, Berlin, Heidelberg, 2009. doi: 10.1007/978-3-642-02971-4\_8 2
